# Supplementary material for: Cross-dimensional Weighting for Aggregated Deep Convolutional Features
Source: arXiv:1512.04065 source file (2016-07-30)
Supplement: Supplementary file 1 [file appendix.tex]

\noindent
\section{What are the image regions that contribute to sparse versus non-sparse channels?} 
To provide further insight into the effect of our sparsity-sensitive channel weights (SSW), we visualize the receptive fields of active locations in channels that our weights boost.

In the right column of Figure~\ref{fig:idf} we show all receptive fields that are non-zero in (one or more) of the channels with the highest sparsity-sensitive channel weights. As values from these channels are increased before aggregation, our approach gives more weight to CNN outputs that correspond to the image regions shown on the right.

Drawing image regions that correspond to non-zero locations in the two channels with the lowest sparsity sensitive weights gave the complete image in all four examples. Therefore, practically the whole image contributes to such channels.

%------------------------------------------------------------------------------
\begin{figure}[ht]
	\centering
    	\foreach \i in {paris_notredame_000035, paris_notredame_000107, paris_pantheon_000014, paris_pantheon_000013} {
		\includegraphics[width=3.9cm]{fig/\i.jpg} \hspace{.3cm} 
		\includegraphics[width=3.9cm]{fig/\i_top_patches_all.jpg} \\ \vspace{.5cm}
    }
\caption{Left: The sample images from Paris dataset (also shown in Figure 3 in the main text). Right: Image regions corresponding to locations that contribute (are non-zero) to the $10$ channels with the highest sparsity-sensitive weights.}
\label{fig:idf}
\end{figure}
%------------------------------------------------------------------------------

% \section{Sparsity figure}

% \section{Spatial Weighting for Saliency Estimation}

\section{Search Results with \Crow Features}

In the following Figures we present search results for the Paris dataset using the \Crow features.
We present the top-10 results returned with the query image and bounding box shown on the leftmost column. The fact that the queries are cropped is the reason why the image where the query comes from is not always returned in the first position.

In Figure~\ref{fig:res} we show the top-10 results for \textit{all} 55 queries on the paris dataset using the uncompressed \Crow features ($d=512$). \textbf{We only have 3 false results in total} for precision@10. This illuminates why query expansion further increases performance: the top ranked results are of high quality.

In Figure~\ref{fig:respatches} we visualize spatial weight maps for the top ten results of a query in $d=512$ dimensions. The ability of the weight maps to boost locations that contain important objects in the scene despite large variations in scale suggests that \Crow features have good scale invariance properties.

In Figure~\ref{fig:resgood} we present some interesting results \emph{using just $d=32$ dimensional features}. They demonstrate the invariance of \Crow features to viewpoint and lighting variations even after heavy compression.
% The third row especially shows that small local variations can be captured in our global representation.

%------------------------------------------------------------------------------
\begin{figure*}[t]
	\centering
		\includegraphics[width=.4\linewidth]{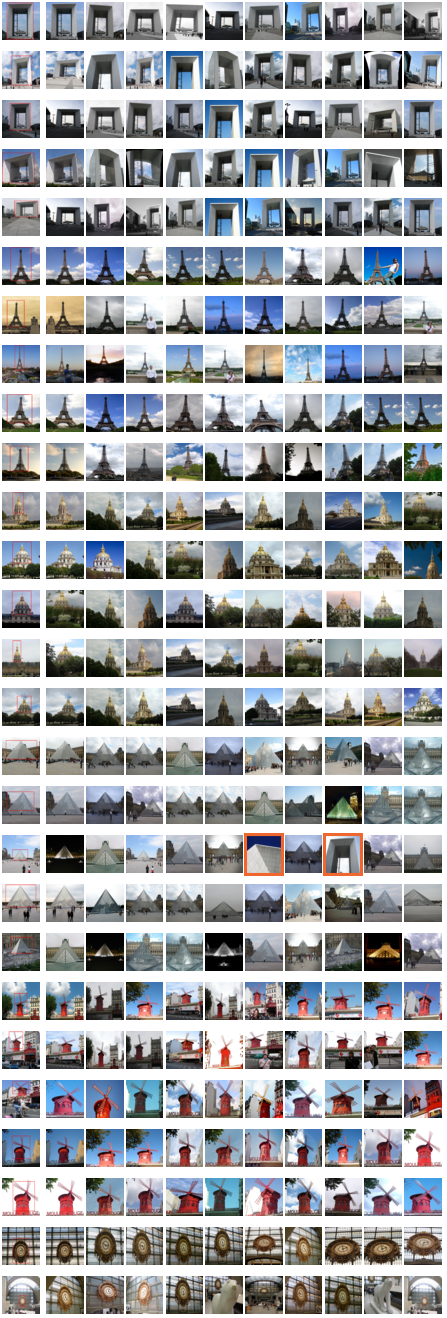} 
		\includegraphics[width=.4\linewidth]{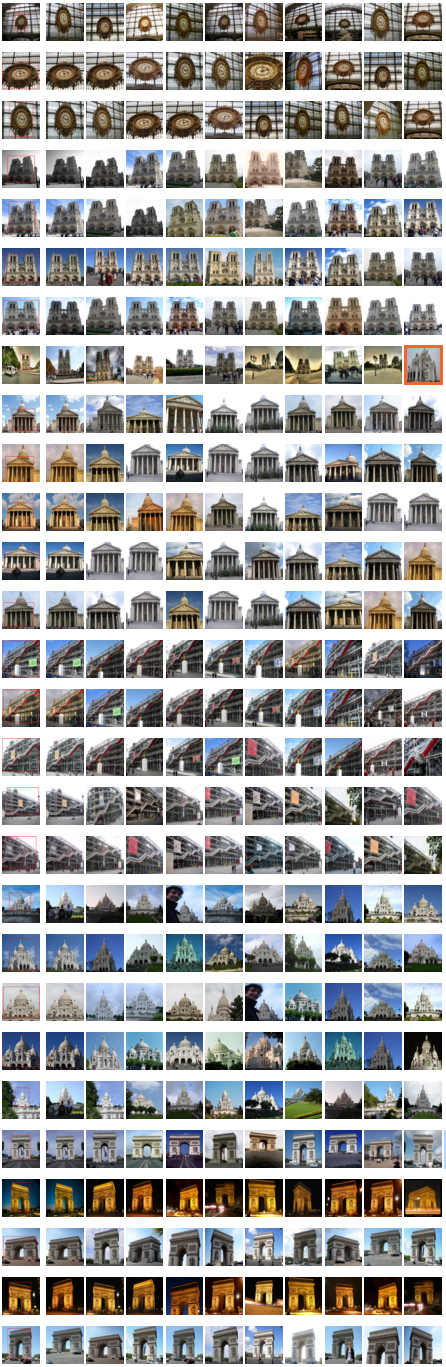} 
        
\caption{Top-10 results returned for all 55 queries of the Paris dataset, using the 512-dimensional \Crow features (and no query expansion). The query image is shown on the leftmost place, with the query bounding box marked with a red rectangle. Our features produce just 3 false results in total, which are marked with an orange border.}
\label{fig:res}
\end{figure*}
%------------------------------------------------------------------------------

%------------------------------------------------------------------------------
\begin{figure*}
	\centering
		\includegraphics[width=\linewidth]{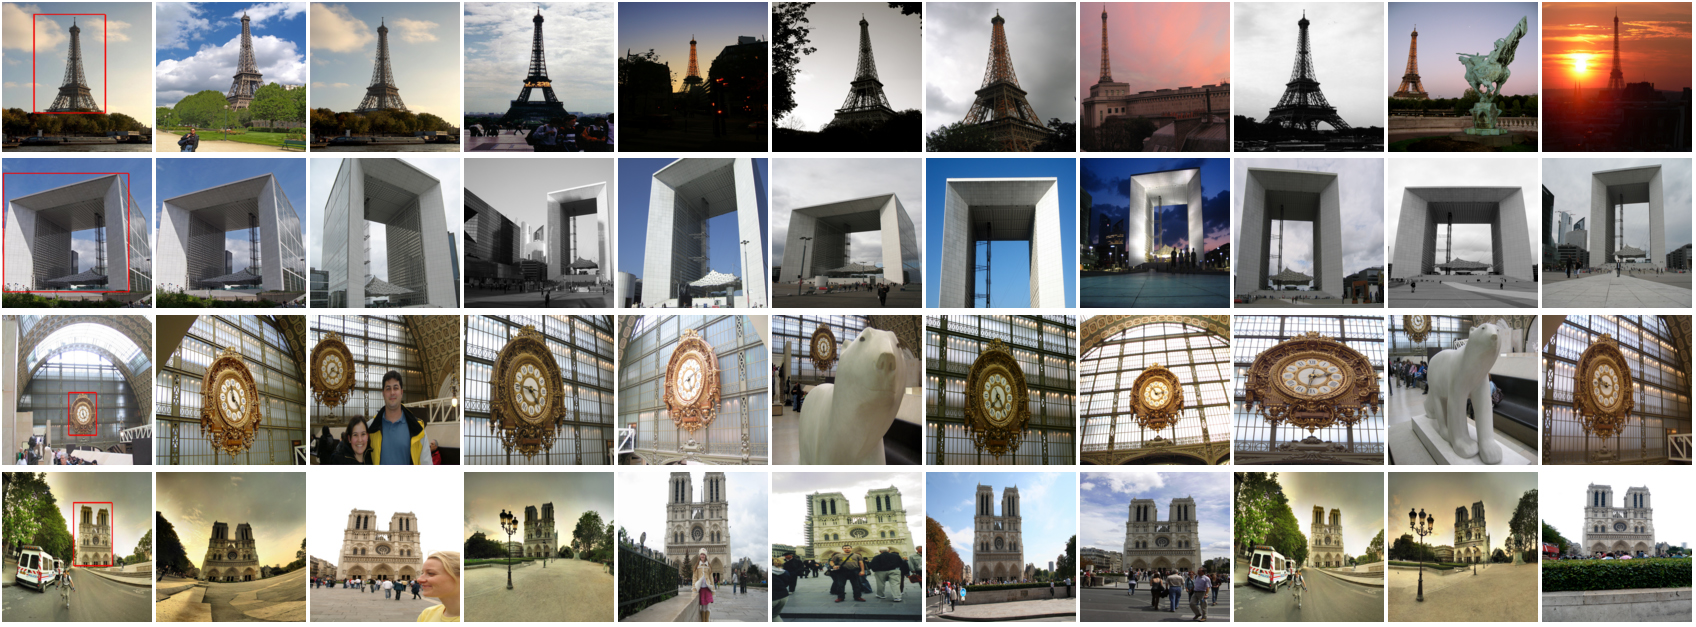} 
\caption{Sample search results using \Crow features compressed to just $d=32$ dimensions. The query image is shown at the leftmost side with the query bounding box marked in a red rectangle.}
\label{fig:resgood}
\end{figure*}
%------------------------------------------------------------------------------

%------------------------------------------------------------------------------
\begin{figure*}
	\centering
		\includegraphics[width=\linewidth]{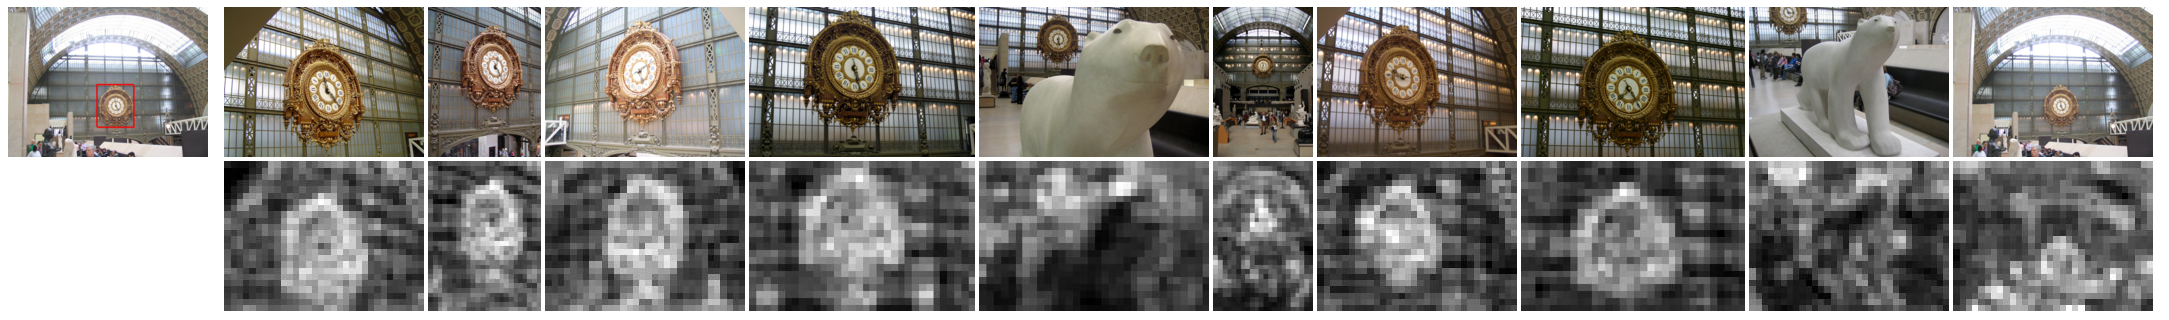} 
\caption{A sample search result using \Crow features with $d=512$ dimensions. Below each result is the corresponding spatial weight map. The query image is shown at the leftmost side with the query bounding box marked in a red rectangle.}
\label{fig:respatches}
\end{figure*}
%------------------------------------------------------------------------------
